# Supplementary material for: Accurate Retraining-free Pruning for Pretrained Encoder-based Language Models
Source: arXiv:2308.03449 source file (2024-03-15)
Supplement: Supplementary file 1 [file appendix.tex]

\documentclass{article}

% if you need to pass options to natbib, use, e.g.:
%     \PassOptionsToPackage{numbers, compress}{natbib}
\PassOptionsToPackage{square,numbers}{natbib}
% before loading neurips_2023

% ready for submission
\bibliographystyle{abbrvnat}
\usepackage{neurips_2023_appendix}

% to compile a preprint version, e.g., for submission to arXiv, add add the
% [preprint] option:
%     \usepackage[preprint]{neurips_2023}

% to compile a camera-ready version, add the [final] option, e.g.:
%     \usepackage[final]{neurips_2023}

% to avoid loading the natbib package, add option nonatbib:
%    \usepackage[nonatbib]{neurips_2023}

%%%%%%%%%%%% Mathcommand for equations %%%%%%%%%
\input{math_commands.tex}

%%%%%%%%%%%%%%%%%% Base packages %%%%%%%%%%%%%%%%%%%%%%
\usepackage[utf8]{inputenc} % allow utf-8 input
\usepackage[T1]{fontenc}    % use 8-bit T1 fonts
\usepackage{hyperref}       % hyperlinks
\usepackage{url}            % simple URL typesetting
\usepackage{booktabs}       % professional-quality tables
\usepackage{multirow}
\usepackage{amsfonts}       % blackboard math symbols
\usepackage{nicefrac}       % compact symbols for 1/2, etc.
\usepackage{microtype}      % microtypography
\usepackage[dvipsnames]{xcolor}         % colors

%%%%%%%%%%%%%%%%%%%%%%% My Packages %%%%%%%%%%%%%%%%%%%
\usepackage{booktabs}
\usepackage{graphicx}
\usepackage{xspace}
\usepackage{amsmath}
\usepackage{bbm} % For one vector
\usepackage{subcaption}
\usepackage{algorithm}
\usepackage{algpseudocode}
\usepackage{mdwlist}
% \usepackage{unicode-math} % for bbold 1
%\usepackage{floatrow} % for Figure 3 and Table 3
%\newfloatcommand{capbtabbox}{table}[][\FBwidth]
%\usepackage{blindtext}

%%%%%%%%%%%%%%%%%%%%%%% My Commands %%%%%%%%%%%%%%%%%%%
%\newcommand{\red}{\textcolor{red}}
%\newcommand{\blue}{\textcolor{blue}}
%\newcommand{\orange}{\textcolor{orange}}
%\newcommand{\green}{\textcolor{OliveGreen}}

% Bold symbols

%

%

% For checkmark and xmark
\usepackage{pifont}% http://ctan.org/pkg/pifont
%
%

%% For appendix numberring
%\setcounter{table}{3}
%\setcounter{figure}{3}
%\setcounter{algorithm}{1}
%\setcounter{equation}{13}

% \theoremstyle{definition}

% Citation with brackets

\title{Supplementary Material: \\Knowledge-preserving Pruning for \\Pre-trained Language Models without Retraining}
% \title{An Efficient Pruning of Pre-trained Language Models}

% The \author macro works with any number of authors. There are two commands
% used to separate the names and addresses of multiple authors: \And and \AND.
%
% Using \And between authors leaves it to LaTeX to determine where to break the
% lines. Using \AND forces a line break at that point. So, if LaTeX puts 3 of 4
% authors names on the first line, and the last on the second line, try using
% \AND instead of \And before the third author name.

%\author{%
%  David S.~Hippocampus\thanks{Use footnote for providing further information
%    about author (webpage, alternative address)---\emph{not} for acknowledging
%    funding agencies.} \\
%  Department of Computer Science\\
%  Cranberry-Lemon University\\
%  Pittsburgh, PA 15213 \\
%  \texttt{hippo@cs.cranberry-lemon.edu} \\
%  % examples of more authors
%  % \And
%  % Coauthor \\
%  % Affiliation \\
%  % Address \\
%  % \texttt{email} \\
%}

\begin{document}

\maketitle

\appendix
\input{099appendix}

\newpage
\bibliography{reference}

%\section{Appendix}
%\label{sec:appendix}
%\input{099appendix}

\end{document}
